# Supplementary material for: Search for the lepton-flavor violating decay $B^0_s\to\phi\mu^\pm\tau^\mp$
Source: arXiv:2405.13103 source file (2024-11-18)
Supplement: Supplementary file 1 [file appendix.tex]

% ===============================================================================
% Purpose: appendix to the standard template: standard symbol alises from Ulrik
% Author: Tomasz Skwarnicki
% Created on: 2009-09-24
% ===============================================================================

%{\noindent\normalfont\bfseries\Large Appendices}
\section*{Appendices}

\appendix
