# Supplementary material for: Search for the lepton-flavor violating decay $B^0_s\to\phi\mu^\pm\tau^\mp$
Source: arXiv:2405.13103 source file (2024-11-18)
Supplement: Supplementary file 3 [file supplementary.tex]

\section{Inclusion of supplementary material}
\label{sec:Supplementary}
